# Supplementary material for: Exploring Functional Photonic Devices made from a Chiral Metal-Organic Framework Material by a Multiscale Computational Method
Source: arXiv:2302.01767 ancillary file (2023-02-03)
Supplement: Supplementary file 1 [file Supporting_Information.pdf]

# Supporting information: Exploring Functional Photonic Devices made from a Chiral Metal-Organic Framework Material by a Multiscale Computational Method

Benedikt Zerulla,[1] Chun Li,[2] Dominik Beutel,[3] Simon Oßwald,[4] Christof Holzer,[3] Jochen Bürck,[5] S. Bräse,[4,6] Christof Wöll,[2] Ivan Fernandez-Corbaton,[1] Lars Heinke*,[2] Carsten Rockstuhl*,[1,3] and Marjan Krstić*[3]

[1)] *Institute of Nanotechnology, Karlsruhe Institute of Technology (KIT), 76344 Eggenstein-Leopoldshafen, Germany*

[2)] *Institute of Functional Interfaces Karlsruhe Institute of Technology (KIT) 76344 Eggenstein-Leopoldshafen, Germany*

[3)] *Institute of Theoretical Solid State Physics, Karlsruhe Institute of Technology (KIT), 76131 Karlsruhe, Germany*

[4)] *Institute of Organic Chemistry, Karlsruhe Institute of Technology (KIT), 76131 Karlsruhe, Germany*

[5)] *Institute of Biological Interfaces (IBG-2), Karlsruhe Institute of Technology (KIT), 76344 Eggenstein-Leopoldshafen, Germany*

[6)] *Institute of Biological and Chemical Systems–Functional Molecular Systems, Karlsruhe Institute of Technology (KIT), 76344 Eggenstein-Leopoldshafen, Germany*

(Dated: 30 January 2023)

## I. COMPUTATIONAL METHODS

The unit cell of the periodic UiO-67-*R*-BINOL MOF was optimized using the periodic DFT code CP2K 7.1.[1] The PBE functional in combination with Grimme's D3 dispersion correction with Becke-Johnson damping was also employed to account for the long-range inter-molecular interactions which additionally stabilized the final structure. Molecular orbitals and electronic density were constructed from DZVP-MOLOPT-GTH[2] basis set and GTH-PBE potentials[3–5]. The cutoff value was set at 600 Ry with SCF energy convergence criteria of 3.0e-6. The unit cell exhibits FCU topology and all three optimized lattice vectors $\boldsymbol{a}$, $\boldsymbol{b}$ and $\boldsymbol{c}$, were found to be 27.647106 Ångströms. The quality of the optimized structure was confirmed comparing the simulated X-Ray diffractogram of the material with the experimental measurements in Figure 1(b) of the manuscript.

Subsequently, the optimized periodic unit cell was used as a base to construct the finite-size molecular model where all broken covalent bonds at the boundary of the unit cell have been saturated with hydrogen atoms. The molecular model consists of 1074 atoms in total and was used for TD-DFT calculation of dynamic polarizabilities for discrete wavelengths in the range from 190-400 nm and the step of 2 nm. The modified Turbomole[6] DFT software was employed for those calculations. The combination of the PBE[7,8] functional and def2-SVP[9] basis set was used for all atoms, while Zr atoms also had Stuttgart effective core potential to speed-up the calculations. An additional speed-up was achieved by enabling resolution-of-identity (RI)[10] and multipole-accelerated RI-J[11] algorithms. The damping was set to 0.15 eV for half-width at half-maximum (HWHM) of the Lorentzian line-shape to match the experimental ECD spectra broadening. In Figure 2 of the manuscript, one can observe that experimental measurements for ECD exhibit a broader spectrum compared to UV-Vis spectrum. A similar behavior was also observed for other MOF materials. We speculate that this stems from the fact that many closed transitions are present in the spectra in that wavelength frame which contributes to such behavior. In total, 106 points were calculated and used for the reconstruction of the UV-Vis and ECD spectra as well as ffor the construction of T-matrices for multi-scale simulations. The T-matrices for the chiral S-enantiomer of the molecular model were constructed by mirroring operations over the XZ-plane which reduced the expensive TD-DFT computational cost to only one molecular model. For the direct comparison of the ECD spectra between the TD-DFT simulations of the molecular model of the MOF material and the experimental measurements of MOF thin films in Figure 2(b), we switched

the labelings of the UiO-67-BINOL measurements.

## II. EXPERIMENTAL METHODS

The reactions were performed according to several literature-reported procedures with slight modifications. The analytical data are in accordance with the reported literature.[12–15]

### A. (Z)-N,6-dimethoxy-3,4-dihydro-2H-naphthalen-1-imine (2)

6-Methoxytetralin-1-one (26.4 g, 150 mmol, 1.00 equiv) and methoxyammoniumchloride (25.1 g, 300 mmol, 2.00 equiv) were dissolved in ethanol (300 mL) under an argon atmosphere. Pyridine (30.0 mL) wasadded, and the mixture was degassed by bubbling with argon for 5 min and then heated to reflux for 1 hour. The solution was concentrated under reduced pressure; dichloromethane (100 mL) was added; the mixture was acidified with hydrochloric acid (2M aq. sol.). The organic phase was separated,and the aqueous phase was extracted with dichloromethane (2 x 100 mL). The combined organic layers were washed with $NaHCO_3$ (1M aq. sol., 50 mL) and brine (50 mL), dried over $Na_2SO_4$, filtered, and the solvent was evaporated under reduced pressure. (Z)-N,6-dimethoxy-3,4-dihydro-2H-naphthalen-1-imine(**2**) (30.4 g, 148 mmol, 99% yield) was obtained as a slightly greenish oil.

$\mathbf{R_f}$(CH/EtOAc, 10:1) = 0.54. – $^1$**H NMR** (400 MHz, $CDCl_3$, ppm) δ = 7.91 (d, *J* = 8.8 Hz, 1H, $H_{Ar}$), 6.75 (dd, *J* = 8.8, 2.7 Hz, 1H,. $H_{Ar}$), 6.63 (d, *J* = 2.7 Hz, 1H, $H_{Ar}$), 3.96 (s, 3H, $OCH_3$), 3.81 (s, 3H, $OCH_3$), 2.75–2.67 (m, 4H, $CH_2$), 1.89–1.78 (m, 2H,$CH_2$). –$^{13}$**C NMR** (101 MHz, $CDCl_3$, ppm) δ = 160.1 ($C_q$, $C_{Ar}$), 153.9 ($C_q$, $C_{Ar}$), 141.2 ($C_q$, $C_{Ar}$), 125.8 (+, CH, $C_{Ar}$), 123.5 ($C_q$, $C_{Ar}$), 112.9 (+, CH, $C_{Ar}$), 112.7 (+, CH, $C_{Ar}$), 61.8 (+, $CH_3$, $OCH_3$), 55.2 (+, $CH_3$, $OCH_3$), 30.1 (–, $CH_2$, $CH_2$), 24.1 (–, $CH_2$, $CH_2$), 21.5 (–, $CH_2$, $CH_2$). – **MS** (EI, 70 eV, 20 °C), m/z (%): 205 (100) $[M]^+$, 174 (12) $[M – OMe]^+$, 146 (21) $[C_{10}H_{12}N]^+$; HRMS–EI *(m/z)*: $[M]^+$ calcd for $C_{12}H_{15}O_2N$, 205.1097; found, 205.1095. – **IR** (ATR, ṽ) = 2934, 2900, 2870, 2836, 2815, 1613, 1592, 1564, 1497, 1462, 1438, 1350, 1323, 1273, 1248, 1235, 1190, 1157, 1132, 1119, 1075, 1051, 1038, 945, 909, 894, 861, 834, 822, 752, 738, 714, 612, 572, 538, 476, 436 $cm^{-1}$.

Additional information on the reaction details is available via the Chemotion repository: https://dx.doi.org/10.14272/reaction/SA-FUHFF-UHFFFADPSC-VUWWOMAFWY-UHFFFADPSC-NUHFF-NQAQP-NUHFF-ZZZ

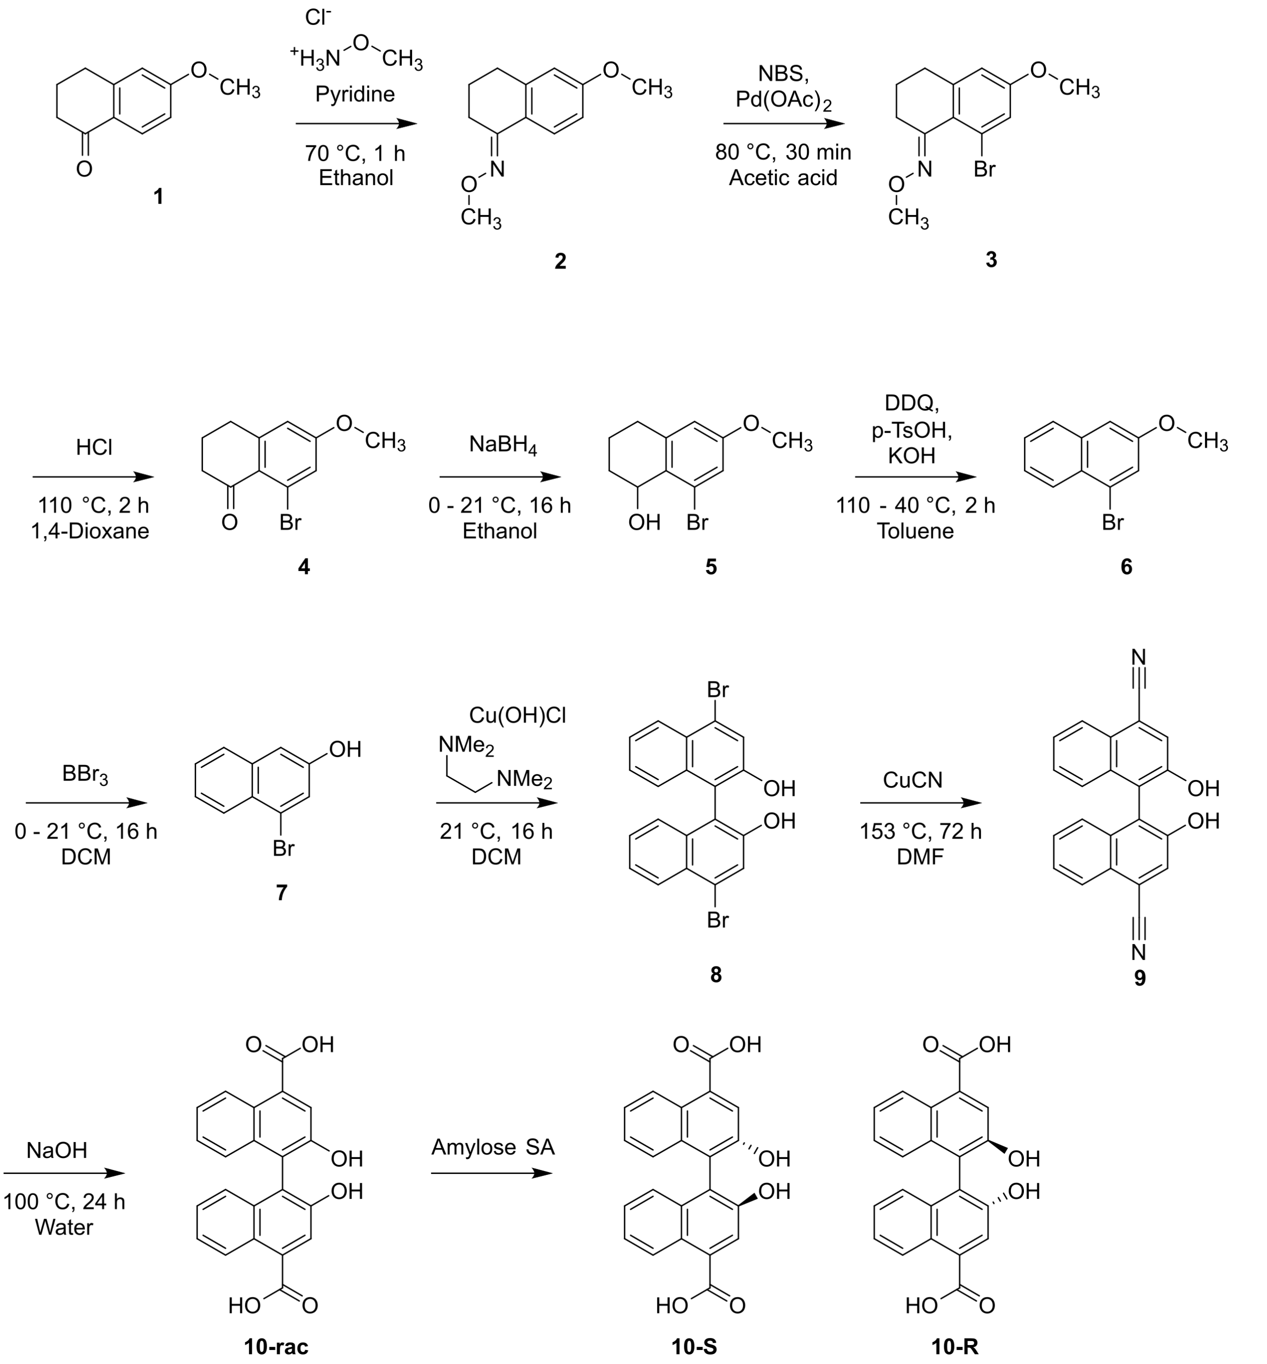


FIG. S1: A step-by-step synthesis scheme of the chiral BINOL linkers used in preparation of the chiral UiO-67-BINOL MOF film material.

Additional information on the analysis of the target compound is available via the Chemotion repository: https://dx.doi.org/10.14272/VUWWOMAFWYFFIK-SEYXRHQNSA-N.1

## B. (E)-8-bromo-6-methoxy-3,4-dihydronaphthalen-1(2H)-one O-methyl oxime (3)

**2** (8.00 g, 39.0 mmol, 1.00 equiv) was dissolved in acetic acid (170 mL). The solution was degassed by bubbling with argon for 10 min. To this solution, N-bromosuccinimide (8.12 g, 45.6 mmol, 1.17 equiv) and palladium(II) acetate (438 mg, 1.95 mmol, 0.0500 equiv) were added, and the mixture was degassed again by bubbling with argon for 10 min. The solution was stirred at 80 °C for 30 min. After cooling to 21 °C, the solution was filtered through Celite and concentrated under reduced pressure. Ethyl acetate (50 mL) and NaHSO3 (sat. aq. sol., 30 mL) were added. The phases were separated, and the aqueous phase was extracted with ethyl acetate (2 x 50 mL). The combined organic layers were washed with $NaHCO_3$ (sat. aq. sol., 30 mL), water (30 mL), and brine (30 mL), dried over $Na_2SO_4$, filtered, and the solvent was evaporated under reduced pressure. The crude product was purified via flash-chromatography (cyclohexane/ethyl acetate 15:1). (E)-8-bromo-6-methoxy-3,4-dihydronaphthalen-1(2H)-one O-methyl oxime (3) (8.17 g, 28.8 mmol, 74% yield) was obtained as a yellowish oil, that gets to solid while storing in the fridge.

$\mathbf{R_f}$(CH/EtOAc, 10:1) = 0.54. – **m.p.**: 61 °C – $^1$**H NMR** (400 MHz, $CDCl_3$, ppm) δ = 7.08 (d, *J* = 2.5 Hz, 1H, $H_{Ar}$), 6.64 (d, *J* = 2.5 Hz, 1H, $H_{Ar}$), 4.01 (s, 3H, $OCH_3$), 3.79 (s, 3H, $OCH_3$), 2.79–2.64 (m, 2H, $CH_2$), 2.63–2.55 (m, 2H, $CH_2$), 1.80–1.68 (m, 2H, $CH_2$). – $^{13}$**C NMR** (101 MHz, $CDCl_3$, ppm) δ = 159.2 ($C_q$, CN), 153.0 ($C_q$, $C_{Ar}$), 144.9 ($C_q$, $C_{Ar}$), 123.7 ($C_q$, $C_{Ar}$), 121.1 ($C_q$, $C_{Ar}$), 118.8 (+, CH, $C_{Ar}$), 113.1 (+, CH, $C_{Ar}$), 62.2 (+, $CH_3$, $OCH_3$), 55.6 (+, $CH_3$, $OCH_3$), 31.5 (–, $CH_2$, $CH_2$), 25.0 (–, $CH_2$, $CH_2$), 21.0 (–, $CH_2$, $CH_2$). – **MS** (EI, 70 eV, 30 °C), m/z (%): 283/285 (100) $[M]^+$, 205 (83) $[M - Br]^+$, 176 (40) $[C_{11}H_{14}NO]^+$, 146 (25) $[C_{10}H_{12}N]^+$; HRMS–EI *(m/z)*: $[M]^+$ calcd for $C_{12}H_{14}O_2N^{79}Br$, 283.0202; found, 283.0202. – **IR** (ATR, ṽ) = 2941, 2893, 2837, 2823, 1604, 1582, 1548, 1466, 1438, 1414, 1350, 1329, 1315, 1292, 1245, 1211, 1191, 1160, 1146, 1123, 1082, 1045, 1034, 966, 948, 916, 907, 870, 844, 833, 809, 795, 782, 751, 720, 673, 630, 618, 591, 574, 547, 526, 479, 456, 429 $cm^1$.

Additional information on the reaction details is available via the Chemotion repository: https://dx.doi.org/10.14272/reaction/SA-FUHFF-UHFFFADPSC-FWRPHJBHZL-UHFFFADPSC-NUHFF-NPCVI-NUHFF-ZZZ

Additional information on the analysis of the target compound is available via the Chemotion repository: https://dx.doi.org/10.14272/FWRPHJBHZLJZOM-SDNWHVSQSA-N.1

## C. 8-bromo-6-methoxy-3,4-dihydro-2H-naphthalen-1-one (4)

**3** (19.9 g, 70.0 mmol, 1.00 equiv) was dissolved in 1,4-dioxane (250 mL), and hydrochloric acid (6M aq. sol., 350 mL) was added. The mixture was degassed by bubbling with argon for 10 min and then heated to reflux for 1 hour. After cooling to 21 °C, the mixture was extracted with ethyl acetate (3 x 100 mL). The combined organic layers were washed with water (50 mL), NaOH (10% aq. sol., 50 mL), and brine (50 mL), dried over $Na_2SO_4$, filtered, and the solvent was evaporated under reduced pressure. The obtained crude product was purified via flash-chromatography (cyclohexane/ethyl acetate 4:1) and following recrystallization from cyclohexane (50 mL). 8-Bromo-6-methoxy-3,4-dihydro-2H-naphthalen-1-one (10.5 g, 41.2 mmol, 59% yield) was obtained as an off-white solid.

$\mathbf{R_f}$(CH/EtOAc, 5:1) = 0.27. – **m.p.**: 88 °C – $^1$**H NMR** (400 MHz, $CDCl_3$, ppm) δ = 7.10 (d, *J* = 2.5 Hz, 1H, $H_{Ar}$), 6.69 (d, *J* = 2.5 Hz, 1H, $H_{Ar}$), 3.84 (s, 3H, $OCH_3$), 2.93 (t, *J* = 6.1 Hz, 2H, $CH_2$), 2.64 (dd, *J* = 7.2, 6.1 Hz, 2H, $CH_2$), 2.12–2.01 (m, 2H, $CH_2$). – $^{13}$**C NMR** (100 MHz, $CDCl_3$, ppm) δ = 195.6 ($C_q$, CO), 162.0 ($C_q$, $C_{Ar}$), 148.9 ($C_q$, $C_{Ar}$), 124.5 ($C_q$, $C_{Ar}$), 123.8 ($C_q$, $C_{Ar}$), 120.0 (+, CH, $C_{Ar}$), 113.3 (+, CH, $C_{Ar}$), 55.8 (+, $CH_3$, $OCH_3$), 40.1 (–, $CH_2$, $CH_2$), 31.7 (–, $CH_2$, $CH_2$), 22.6 (–, $CH_2$, $CH_2$). – **MS** (EI, 70 eV, 40 °C), m/z (%): 254/256 (65) $[M]^+$, 226/228 (100) $[M - CO]^+$; HRMS–EI *(m/z)*: $[M]^+$ calcd for $C_{11}H_{11}O_2{}^{79}Br$, 253.9937; found, 253.9939. – **IR** (ATR, ṽ) = 3074, 3009, 2973, 2945, 2873, 2840, 1674, 1585, 1554, 1456, 1431, 1417, 1347, 1340, 1313, 1264, 1244, 1176, 1119, 1079, 1055, 1037, 1017, 952, 914, 894, 884, 873, 840, 790, 745, 679, 664, 613, 558, 517, 499, 436, 404 $cm^{-1}$.

Additional information on the reaction details is available via the Chemotion repository: https://dx.doi.org/10.14272/reaction/SA-FUHFF-UHFFFADPSC-DTGKGALXLO-UHFFFADPSC-NUHFF-NUHFF-NUHFF-ZZZ

Additional information on the analysis of the target compound is available via the Chemotion repository: https://dx.doi.org/10.14272/DTGKGALXLOFBAY-UHFFFAOYSA-N.1

## D. 8-bromo-6-methoxy-1,2,3,4-tetrahydronaphthalen-1-ol (5)

8-Bromo-6-methoxy-3,4-dihydro-2H-naphthalen-1-one (10.2 g, 40.0 mmol, 1.00 equiv) was dissolved in ethanol (75.0 mL) and cooled to 0 °C. The mixture was degassed by bubbling with argon for 10 min. Sodium borohydride (3.03 g, 80.0 mmol, 2.00 equiv) was added portionwise,

and the reaction was allowed to warm slowly to 21 °C and stirred for 16 hours. NH4Cl (sat. aq. sol., 50 mL) was added, and the mixture was extracted with dichloromethane (3 x 50 mL). The combined organic layers were washed with water (50 mL) and brine (50 mL), dried over $Na_2SO_4$, filtered, and the solvent was evaporated under reduced pressure. 8-Bromo-6-methoxy-1,2,3,4-tetrahydronaphthalen-1-ol (10.0 g, 39.0 mmol, 98% yield) was obtained as a white crystalline solid.

**$R_f$**(CH/EtOAc, 2:1) = 0.54. – **m.p.**: 99 °C – **$^1$H NMR** (400 MHz, $CDCl_3$, ppm) δ = 7.00 (d, *J* = 2.5 Hz, 1H, $H_{Ar}$), 6.62 (d, *J* = 2.5 Hz, 1H, $H_{Ar}$), 4.97 (q, *J* = 3.4 Hz, 1H, OH), 3.77 (s, 3H, $OCH_3$), 2.90–2.75 (m, 1H, $CH_2$), 2.75–2.61 (m, 1H, CHOH), 2.29 (dd, *J* = 3.7, 1.3 Hz, 1H, $CH_2$), 2.22–2.13 (m, 1H, $CH_2$), 2.06–1.88 (m, 1H, $CH_2$), 1.81–1.66 (m, 2H, $CH_2$). – **$^{13}$C NMR** (100 MHz, $CDCl_3$, ppm) δ = 159.2 ($C_q$, $C_{Ar}$), 141.1 ($C_q$, $C_{Ar}$), 129.8 ($C_q$, $C_{Ar}$), 126.3 ($C_q$, $C_{Ar}$), 116.8 (+, CH, $C_{Ar}$), 113.9 (+, CH, $C_{Ar}$), 65.9 (+, CH, CHOH), 55.6 (+, $CH_3$, $OCH_3$), 31.2 (–, $CH_2$, $CH_2$), 30.4 (–, $CH_2$, $CH_2$), 17.4 (–, $CH_2$, $CH_2$). – **MS** (EI, 70 eV, 40 °C), m/z (%): 256/258 (12) $[M]^+$, 238/240 (25) $[M – H2O]^+$, 178 (50), 177 (66) $[M – Br]^+$, 160 (100) $[C_{11}H_{12}O]^+$, 159 (58) $[C_{11}H_{11}O]^+$, 158 (18), 150 (35), 149 (34), 147 (22), 145 (29), 144 (31), 115 (63); HRMS–EI *(m/z)*: $[M]^+$ calcd for $C_{11}H_{13}O_2{}^{79}Br$, 256,0093; found, 256,0095. – **IR** (ATR, ṽ) = 3166, 2942, 2912, 2833, 1599, 1564, 1468, 1265, 1261, 1242, 1116, 1077, 1040, 1014, 965, 925, 854, 832, 806, 703, 472 $cm^{-1}$.

Additional information on the reaction details is available via the Chemotion repository: https://dx.doi.org/10.14272/reaction/SA-FUHFF-UHFFFADPSC-AEXVLWUCIQ-UHFFFADPSC-NUHFF-NUHFF-NUHFF-ZZZ

Additional information on the analysis of the target compound is available via the Chemotion repository: https://dx.doi.org/10.14272/AEXVLWUCIQKDMV-UHFFFAOYSA-N.1

### E. 1-Bromo-3-methoxynaphthalene (6)

8-Bromo-6-methoxy-1,2,3,4-tetrahydronaphthalen-1-ol (9.51 g, 37.0 mmol, 1.00 equiv) was dissolved in toluene (190 mL). p-Toluenesulfonic acid monohydrate (704 mg, 3.70 mmol, 0.100 equiv) was added, and the mixture was degassed by bubbling with argon for 5 min and heated to reflux for 30 min. After cooling to 21 °C, powdered potassium hydroxide (208 mg, 3.70 mmol, 0.100 equiv) was added, and the mixture was stirred for 10 min. DDQ (10.9 g, 48.1 mmol, 1.30 equiv) was added, and the reaction was stirred at 40 °C for 2 hours. The solvent was evaporated

under reduced pressure, and the residue was resuspended in dichloromethane/petroleum ether 40-60 (1:4, 50 mL) and filtered through a short plug of Silica. The solvent was evaporated under reduced pressure.1-Bromo-3-methoxynaphthalene (7.16 g, 30.2 mmol, 82% yield) was obtained as an off-white solid.

**$R_f$**(CH/EtOAc, 10:1) = 0.56. – **m.p.**: 64 °C – **$^1$H NMR** (400 MHz, $CDCl_3$, ppm) δ = 8.14 (d, $J$ = 7.8 Hz, 1H, $H_{Ar}$), 7.72 (d, $J$ = 7.8 Hz, 1H, $H_{Ar}$), 7.50 (d, $J$ = 2.5 Hz, 1H, $H_{Ar}$), 7.49–7.41 (m, 2H, $H_{Ar}$), 7.12 (d, $J$ = 2.4 Hz, 1H, $H_{Ar}$), 3.91 (s, 3H, $OCH_3$). – **$^{13}$C NMR** (100 MHz, $CDCl_3$, ppm) δ = 157.3 ($C_q$, $C_{Ar}$), 135.3 ($C_q$, $C_{Ar}$), 127.8 (+, CH, $C_{Ar}$), 127.3 (+, CH, $C_{Ar}$), 127.3 (+, CH, $C_{Ar}$), 127.1 ($C_q$, $C_{Ar}$), 125.1 (+, CH, $C_{Ar}$), 123.6 ($C_q$, $C_{Ar}$), 122.8 (+, CH, $C_{Ar}$), 106.3 (+, CH, $C_{Ar}$), 55.7 (+, $CH_3$, $OCH_3$). – **MS** (EI, 70 eV, 20 °C), m/z (%): 236/238 (100) $[M]^+$, 193/195 (53) $[C_9H_6Br]^+$, 127 (15) $[C_{10}H_{11}]^+$, 114 (35) $[C_9H_6]^+$; HRMS–EI *(m/z)*: $[M]^+$ calcd for $C_{11}H_9O^{79}Br$, 235.9831; found, 235.9833. – **IR** (ATR, ṽ) = 3061, 2993, 2962, 2939, 2864, 2833, 1623, 1598, 1565, 1500, 1460, 1449, 1422, 1383, 1357, 1344, 1259, 1225, 1194, 1167, 1149, 1125, 1040, 1021, 984, 972, 953, 945, 904, 880, 860, 832, 822, 759, 738, 725, 635, 565, 560, 514, 475, 449, 418 $cm^{-1}$.

Additional information on the reaction details is available via the Chemotion repository: https://dx.doi.org/10.14272/reaction/SA-FUHFF-UHFFFADPSC-GPVSVDNPAV-UHFFFADPSC-NUHFF-NUHFF-NUHFF-ZZZ

Additional information on the analysis of the target compound is available via the Chemotion repository:https://dx.doi.org/10.14272/GPVSVDNPAVXAQT-UHFFFAOYSA-N/CHMO0000593

## F. 4-Bromonaphthalen-2-ol (7)

1-Bromo-3-methoxynaphthalene (7.00 g, 29.5 mmol, 1.00 equiv) was dissolved in dichloromethane (70.0 mL), the mixture was degassed by bubbling with argon and cooled to 0 °C. Tribromoborane (1M in dichloromethane, 8.88 g, 3.36 mL, 35.4 mmol, 1.20 equiv) was added dropwise over 10 min, and the reaction was allowed to warm to 21 °C and stirred for 16 hours. The reaction was then cooled to 0 °C and quenched by dropwise addition of water (20 mL). The resulting biphasic mixture was extracted with dichloromethane (3 x 50 mL). The combined organic layers were washed with water (50 mL) and brine (50 mL), dried over $Na_2SO_4$, filtered, and the solvent was evaporated under reduced pressure. 4-Bromonaphthalen-2-ol (6.39 g, 28.6 mmol, 99% yield) was obtained as a colorless solid.

**$R_f$**(CH/EtOAc, 10:1) = 0.15. – **m.p.**: 121 °C – **$^1$H NMR** (400 MHz, $CDCl_3$, ppm) δ = 8.16–8.13 (m, 1H, $H_{Ar}$), 7.69–7.66 (m, 1H, $H_{Ar}$), 7.50–7.42 (m, 3H, $H_{Ar}$), 7.15 (d, $J$ = 2.5 Hz, 1H, $H_{Ar}$), 5.10 (s, 1H, OH). – **$^{13}$C NMR** (100 MHz, $CDCl_3$, ppm) δ = 152.9 ($C_q$, $C_{Ar}$), 135.1 ($C_q$, $C_{Ar}$), 127.6 ($C_q$, $C_{Ar}$), 127.4 (+, CH, $C_{Ar}$), 127.0 (+, CH, $C_{Ar}$), 126.9 (+, CH, $C_{Ar}$), 125.0 (+, CH, $C_{Ar}$), 123.7 ($C_q$, CH, $C_{Ar}$), 121.9 (+, CH, $C_{Ar}$), 109.8 (+, CH, $C_{Ar}$). – **MS** (EI, 70 eV, 20 °C), m/z (%): 222/224 (84) $[M]^+$, 144 (47) $[M - Br]^+$, 115 (100) $[C_9H_6]^+$; HRMS–EI *(m/z)*: $[M]^+$ calcd for $C_{10}H_7O^{79}Br$, 221.9675; found, 221.9676. – **IR** (ATR, ṽ) = 3282, 3061, 1629, 1564, 1506, 1435, 1276, 1251, 1228, 1170, 1145, 1123, 915, 840, 823, 759, 737, 629, 510, 424 $cm^{-1}$.

Additional information on the reaction details is available via the Chemotion repository: https://dx.doi.org/10.14272/reaction/SA-FUHFF-UHFFFADPSC-PQNQMYMGUX-UHFFFADPSC-NUHFF-NUHFF-NUHFF-ZZZ

Additional information on the analysis of the target compound is available via the Chemotion repository: https://dx.doi.org/10.14272/PQNQMYMGUXGWTG-UHFFFAOYSA-N.1

## G. Rac-4-Bromo-1-(4-bromo-2-hydroxynaphthalen-1-yl)naphthalen-2-ol (8)

4-Bromonaphthalen-2-ol (6.25 g, 28.0 mmol, 1.00 equiv) was dissolved in dichloromethane (150 mL), and chlorocopper2-(dimethylamino)ethyl-dimethyl-amine (32.5 mg, 140 µmol, 0.0050 equiv) was added. The reaction was stirred at 21 °C for 16 hours open to the air. The reaction mixture was filtered through a short plug of silica eluting with dichloromethane. The solvent was evaporated under reduced pressure. 4-Bromo-1-(4-bromo-2-hydroxynaphthalen-1-yl)naphthalen-2-ol (5.99 g, 13.5 mmol, 96% yield) was obtained as a yellow crystalline solid.

**$R_f$**(CH/EtOAc, 5:1) = 0.41. – **m.p.**: 175 °C – **$^1$H NMR** (400 MHz, $CDCl_3$, ppm) δ = 8.30 (dt, $J$ = 8.4, 1.0 Hz, 2H, $H_{Ar}$), 7.75 (s, 2H, $H_{Ar}$), 7.49 (ddd, $J$ = 8.3, 6.8, 1.2 Hz, 2H, $H_{Ar}$), 7.36 (ddd, $J$ = 8.3, 6.8, 1.3 Hz, 2H, $H_{Ar}$), 7.14 (dt, $J$ = 8.4, 0.9 Hz, 2H, $H_{Ar}$), 5.03 (s, 2H, OH). – **$^{13}$C NMR** (101 MHz, $CDCl_3$, ppm) δ = 152.5 ($C_q$, 2C, $C_{Ar}$), 134.0 ($C_q$, 2C, $C_{Ar}$), 128.6 (+, 2C, CH, $C_{Ar}$), 128.3 ($C_q$, 2C, $C_{Ar}$), 128.0 (+, 2C, CH, $C_{Ar}$), 126.1 ($C_q$, 2C, $C_{Ar}$), 125.7 (+, 2C, CH, $C_{Ar}$), 124.6 (+, 2C, CH, $C_{Ar}$), 122.1 (+, 2C, CH, $C_{Ar}$), 110.6 ($C_q$, 2C, $C_{Ar}$). – **MS** (FAB, 3-NBA), m/z: 442/444/446 $[M + H]^+$, 364/366 $[M + H - Br]^+$; HRMS–FAB *(m/z)*: $[M + H]^+$ calcd for $C_{20}H_{12}O_2{}^{79}Br_2$, 441.9199; found, 441.9196. – **IR** (ATR, ṽ) = 3509, 3452, 3286, 3061, 1594, 1571, 1567, 1504, 1370, 1343, 1295, 1258, 1217, 1188, 1173, 1147, 1129, 1085, 932, 915, 870, 840, 823, 758, 738, 683, 663, 632, 595, 555, 521, 510, 501, 449, 416 $cm^{-1}$.

Additional information on the reaction details is available via the Chemotion repository: https://dx.doi.org/10.14272/reaction/SA-FUHFF-UHFFFADPSC-UAOMNDAJRK-UHFFFADPSC-NUHFF-NUHFF-NUHFF-ZZZ

Additional information on the analysis of the target compound is available via the Chemotion repository: https://dx.doi.org/10.14272/UAOMNDAJRKOYII-UHFFFAOYSA-N.1

## H. Rac-4-(4-Cyano-2-hydroxynaphthalen-1-yl)-3-hydroxynaphthalene-1-carbonitrile (9)

4-Bromo-1-(4-bromo-2-hydroxynaphthalen-1-yl)naphthalen-2-ol (5.77 g, 13.0 mmol, 1.00 equiv) and copper(I) cyanide (4.66 g, 52.0 mmol, 4.00 equiv) were dissolved DMF (140 mL), and the mixture was degassed by bubbling with argon for 15 minutes. The mixture was heated with stirring to reflux for 72 hours. The product was extracted with ethyl acetate (3 x 100 mL) (check pH, acidify slightly when needed to pH about 5-6). The combined organic layers were washed with water (50 mL) and brine (50 mL), dried over $Na_2SO_4$, filtered, and the solvent was evaporated under reduced pressure. The obtained crude product was purified via flash-chromatography (cyclohexane/ethyl acetate 2:1 to 1:2). 4-(4-Cyano-2-hydroxynaphthalen-1-yl)-3-hydroxynaphthalene-1-carbonitrile (3.41 g, 10.1 mmol, 78% yield) was obtained as an off-white solid.

$\mathbf{R_f}$(CH/EtOAc, 2:1) = 0.26. – **m.p.**:>300 °C – $^1$**H NMR** (400 MHz, DMSO-d6, ppm) δ = 10.20 (s, 2H, OH), 8.09 (dt, $J$ = 8.4, 1.0 Hz, 2H, $H_{Ar}$), 7.87 (s, 2H, $H_{Ar}$), 7.55 (ddd, $J$ = 8.2, 6.8, 1.2 Hz, 2H, $H_{Ar}$), 7.41 (ddd, $J$ = 8.3, 6.9, 1.3 Hz, 2H, $H_{Ar}$), 7.05 (dt, $J$ = 8.5, 1.0 Hz, 2H, $H_{Ar}$). – $^{13}$**C NMR** (101 MHz, DMSO-d6, ppm) δ = 152.3 ($C_q$, 2C, COH), 133.5 ($C_q$, 2C, $C_{Ar}$), 128.1 (+, 2C, CH, $C_{Ar}$), 126.7 ($C_q$, 2C, $C_{Ar}$), 125.6 (+, 2C, CH, $C_{Ar}$), 125.1 (+, 2C, CH, $C_{Ar}$), 124.6 (+, 2C, CH, $C_{Ar}$), 124.5 (+, 2C, CH, $C_{Ar}$), 121.0 ($C_q$, 2C, $C_{Ar}$), 117.5 ($C_q$, 2C, $C_{Ar}$), 109.9 ($C_q$, 2C, CN). – **MS** (EI, 70 eV, 200 °C), m/z (%): 336 (100) $[M]^+$; HRMS–EI *(m/z)*: $[M]^+$calcd for $C_{22}H_{12}O_2N_2$, 336.0893; found, 336.0893.– **IR** (ATR, ṽ) = 3325, 3072, 2237, 1734, 1615, 1585, 1568, 1511, 1381, 1349, 1292, 1272, 1225, 1210, 1184, 1173, 1150, 1133, 1038, 1027, 1000, 975, 915, 875, 762, 703, 666, 645, 633, 603, 540, 528, 504, 483, 477, 446, 429, 412 $cm^{-1}$.

Additional information on the reaction details is available via the Chemotion repository: https://dx.doi.org/10.14272/reaction/SA-FUHFF-UHFFFADPSC-XDOHQPHWJL-UHFFFADPSC-NUHFF-NUHFF-NUHFF-ZZZ

Additional information on the analysis of the target compound is available via the Chemotion

repository: https://dx.doi.org/10.14272/XDOHQPHWJLGTGD-UHFFFAOYSA-N.1

## I. Rac-4-(4-carboxy-2-hydroxynaphthalen-1-yl)-3-hydroxynaphthalene-1-carboxylic acid (10)

Sodium hydroxide (6M aq. sol., 33.6 g, 140 mL, 840 mmol, 84.0 equiv)was combined with 4-(4-cyano-2-hydroxynaphthalen-1-yl)-3-hydroxynaphthalene-1-carbonitrile (3.36 g, 10.0 mmol, 1.00 equiv) and the mixture was heated to reflux for 24 hours. After cooling to 21 °C, the mixture was acidified with hydrochloric acid (12M aq. sol.). The product was extracted with ethyl acetate (3 x 100 mL). The combined organic layers were washed with water (50 mL) and brine (50 mL), dried over $Na_2SO_4$, filtered, and the solvent was evaporated under reduced pressure. The crude product was purified by recrystallization from cyclohexane/ethyl acetate 2:1 (100 mL). 4-(4-carboxy-2-hydroxynaphthalen-1-yl)-3-hydroxynaphthalene-1-carboxylic acid (3.45 g, 9.22 mmol, 92% yield) was obtained as an off-white solid.

**$R_f$**(EtOAc) = 0.08. – **m.p.**:>300 °C – **$^1$H NMR** (400 MHz, DMSO-d6, ppm) δ = 13.19 (s, 2H, COOH), 9.67 (s, 2H, OH), 8.85–8.78 (m, 2H, $H_{Ar}$), 7.98 (s, 2H, $H_{Ar}$), 7.37 (ddd, $J$ = 8.4, 6.7, 1.4 Hz, 2H, $H_{Ar}$), 7.25 (ddd, $J$ = 8.3, 6.7, 1.3 Hz, 2H, $H_{Ar}$), 7.04–6.96 (m, 2H, $H_{Ar}$). – **$^{13}$C NMR** (101 MHz, DMSO-d6, ppm) δ = 168.5 ($C_q$, 2C, COOH), 151.8 ($C_q$, 2C, COH), 134.3 ($C_q$, 2C, $C_{Ar}$), 128.8 ($C_q$, 2C, $C_{Ar}$), 126.4 (+, 2C, CH, $C_{Ar}$), 125.8 ($C_q$, 2C, $C_{Ar}$), 125.7 (+, 2C, CH, $C_{Ar}$), 124.8 (+, 2C, CH, $C_{Ar}$), 123.9 (+, 2C, CH, $C_{Ar}$), 121.8 (+, 2C, CH, $C_{Ar}$), 120.2 ($C_q$, 2C, $C_{Ar}$). – **MS** (FAB, 3-NBA), m/z: 375 $[M + H]^+$, 374 $[M]^+$; HRMS–FAB *(m/z)*: $[M]^+$ calcd for $C_{22}H_{14}O_6$, 374.0785; found 374.0786. – **IR** (ATR, ṽ) = 3259, 2973, 1681, 1575, 1513, 1405, 1374, 1340, 1282, 1269, 1239, 1217, 1200, 1181, 1152, 1139, 1096, 1040, 894, 793, 776, 745, 724, 708, 666, 628, 611, 586, 470, 436, 419 $cm^{-1}$.

Additional information on the reaction details is available via the Chemotion repository: https://dx.doi.org/10.14272/reaction/SA-FUHFF-UHFFFADPSC-XZPJJIVENU-UHFFFADPSC-NUHFF-NUHFF-NUHFF-ZZZ

Additional information on the analysis of the target compound is available via the Chemotion repository: https://dx.doi.org/10.14272/XZPJJIVENUMRKP-UHFFFAOYSA-N.1

## J. (S)-4-(4-carboxy-2-hydroxynaphthalen-1-yl)-3-hydroxynaphthalene-1-carboxylic acid (10-S)& (R)-4-(4-carboxy-2-hydroxynaphthalen-1-yl)-3-hydroxynaphthalene-1-carboxylic acid (10-R)

Separation of the racemic mixture was performed via prep. HPLC. An Amylose SA chiral column (30x250 mm, 10µm) was used with ethanol in n-hexane (5-95) + 0.1% TFA as eluent. Each run was loaded with 100 mg of the racemic product, while 40 mg of each enantiomer could be isolated with >99% ee. The optical purity was determined by HPLC analysis using anAmylose SA column (n-hexane/ethanol,70:30 + 0.1% TFA, tR: 10.7 min (S), 16.1 min (R)) and optical rotation (S: –62°, R: +62°; c = 1 g/mL, 20°C; THF).

## K. MOF thin films

MOF films were grown via vapor-assisted conversion (VAC).[16] There, a 200 mL Teflon-lined stainless-steel autoclave was used, where Raschig-rings (1 cm×1 cm) were placed on the bottom of the vial to obtain an elevated flat platform for the substrate. $ZrOCl_2$ (2.2 mM/L), S/R-BINOL linker (2.2 mM/L) and acetic acid (420 mM) were dissolved in a mixed solution DMF as the precursor solution. A mixture of 4.2 mL and 0.8 mL acetic acid was filled into the autoclave as vapour source. The pre-treated Au substrates (for SEM and IRRAS) and quartz substrates (for UV and CD) were placed on top of the Raschig-ring and fully coated with 40 µL freshly prepared MOF precursor solution. Then, it was heated at 120 °C for 3 h. After subsequent cooling down to room temperature, the obtained MOF films were dried in a vacuum.

The X-ray diffraction (XRD) of the MOF thin films was recorded using a D8 ADVANCE X-ray diffractometer (BrukerAXS, German) with Cu-K radiation (40 kV, 40 mA, $\lambda$= 0.154 nm) in the range from 3° to 20°.

The electronic circular dichroism (ECD) spectra of the MOF thin film samples in transmission mode were measured with a Jasco J-810 spectropolarimeter at room temperature. Details on the experimental setup and measurements of MOF thin films deposited on quartz glass supports have been described earlier (see SI of ref. 21 of the manuscript).

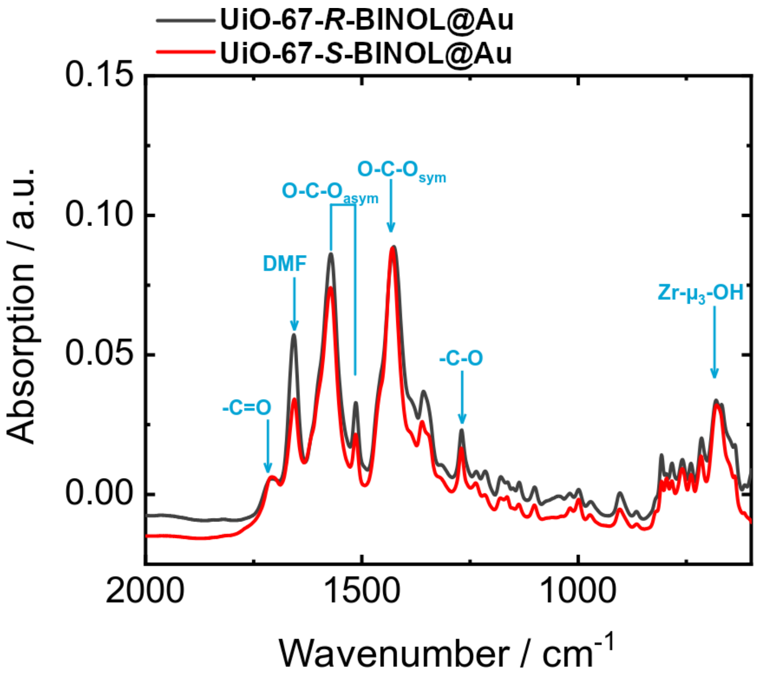


FIG. S2: The IRRA spectra of both eneatiomers of UiO-67-BINOL MOF thin films on the gold substrate.

## III. T-MATRICES FROM TD-DFT CALCULATIONS

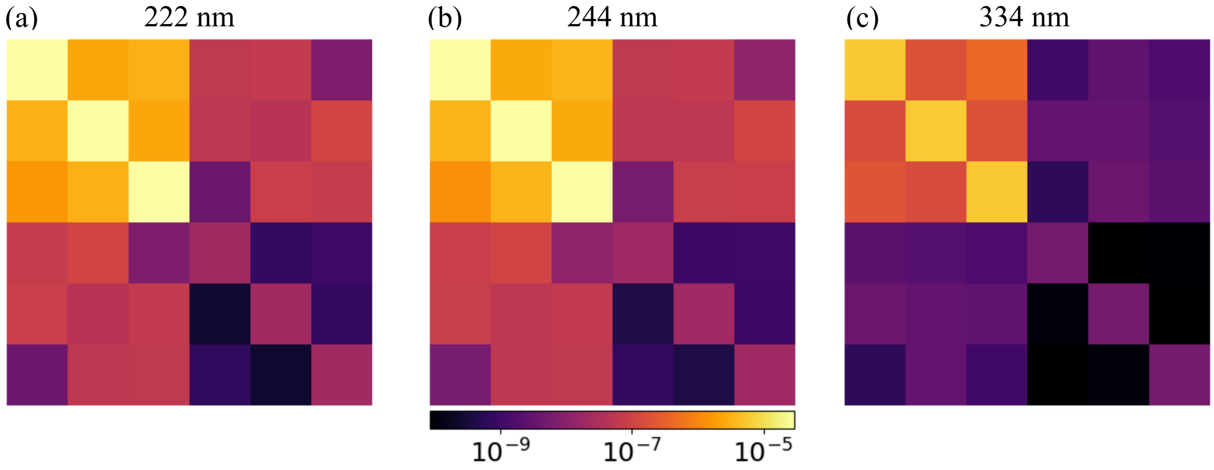


FIG. S3: The visual representation of the T-matrix in parity basis for three chosen wavelengths corresponding to the three distinguished peaks in the simulated ECD spectrum: 222 nm (left), 244 nm (middle) and 334 nm (right). The modulus of the complex values are visualized. The color map scale is the same in all three presented T-matrices.

## IV. SPECTRA OF UIO-*S*-BINOL MOF THIN FILM

In Figure 4 of the main article, we consider the spectra of the circular dichroism of the UiO-*R*-BINOL MOF thin film for different wavelengths of the incident light and different values of the thickness of the MOF film. In Figure S4, the corresponding spectra are shown for the UiO-*S*-BINOL MOF film. As the linkers are of the two MOFs are enantiomers of each other, the corresponding spectra are perfect mirror images. All false-color plots of the ACD and CD spectra in the main article and the SI are plotted with[17].

## V. EFFECTIVE MATERIAL PARAMETERS OF UIO-*R*-BINOL MOF

In Figure S5(**a**) and (**b**), the effective permittivity and chirality are shown, which are calculated for the UiO-*R*-BINOL-MOF with the rotationally averaged unit cell with the homogenization approach from[18]. Both quantities show several resonances. One resonance of the chirality is at 334 nm, which corresponds to the design wavelength of the square lattice of the MOF cylinders from the main article. We do not show the magnetic permeability as it is approximately one throughout the entire frequency range.

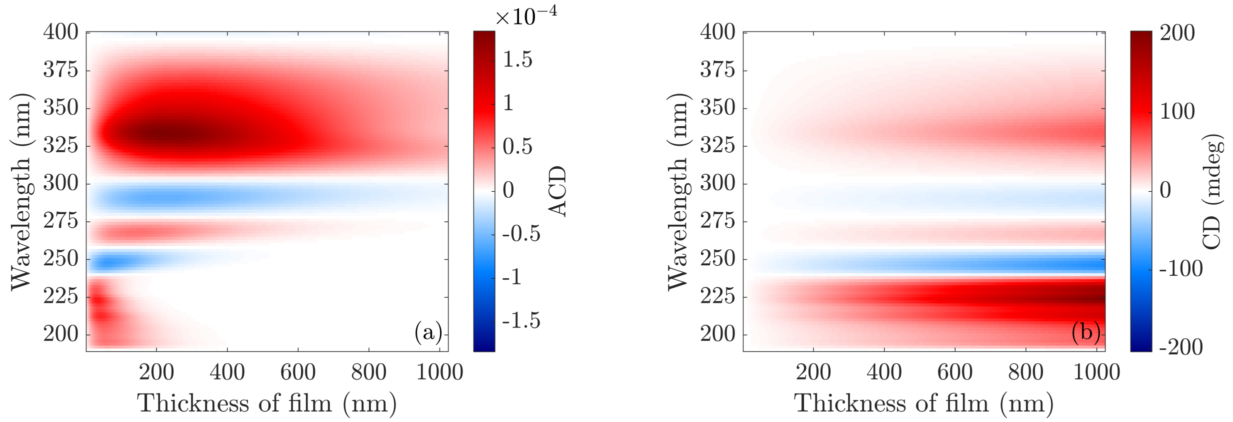


FIG. S4: Absorption circular dichroism (**a**) and transmission circular dichroism (**b**) of the UiO-*S*-BINOL MOF thin film. The spectra are perfect mirror images of the spectra in Figure 4(**b**) and Figure 4(**c**), which show the corresponding quantities for the UiO-*R*-BINOL MOF.

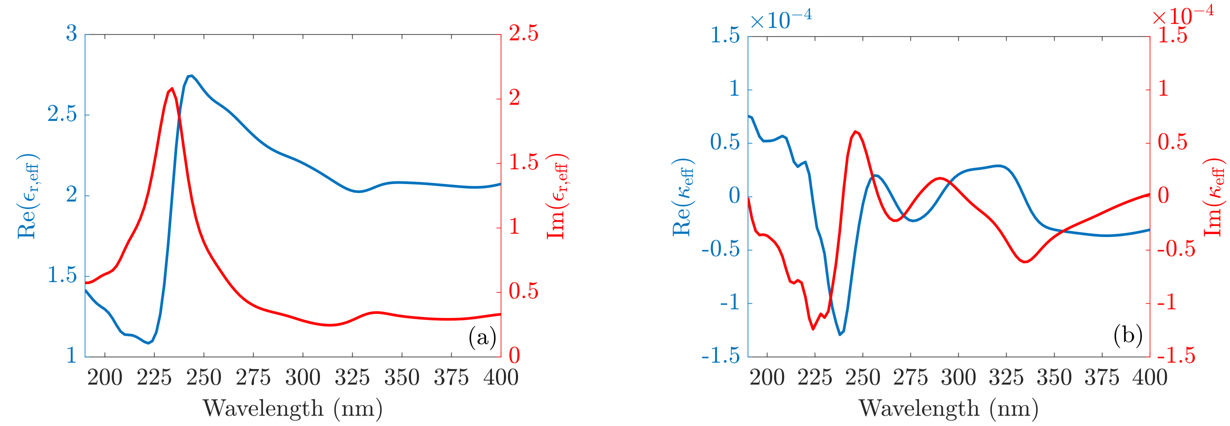


FIG. S5: Effective permittivity **(a)** and chirality **(b)** of the UiO-*R*-BINOL-MOF with rotationally averaged unit cell. The chirality shows a resonance at 334 nm.

## VI. RESPONSE OF MOF THIN FILM WITH ORIENTED UNIT CELLS

We analyze in the following the influence of the structure of the UiO-*R*-BINOL-MOF on the circular dichroism by incorporating the full T-matrix into the multi-scattering problem instead of rotationally averaging the four block matrices of the T-matrix. The orientation of the MOF is chosen as depicted in Figure 3 of the main article. The absorption is shown in Figure S6(**a**), the ACD spectrum is shown in Figure S6(**b**), and the CD spectrum is shown in Figure S6(**c**). One observes in **(a)** that the absorption is very similar to the spectrum of the MOF with rotationally averaged unit cells shown in Figure 4 of the main article. Comparing the ACD spectrum in **(b)** to the CD spectrum in (**c**), we observe that in general both show for the same wavelengths the same sign. A significant characteristic of the spectra is that for wavelengths between 225 nm and 250 nm, both show a change of sign for an approximate thickness of the film of 200 nm. This is not observed for the MOF thin film with rotationally averaged unit cells.

To analyze this specific feature of the circular dichroism spectra of the oriented MOFs, we discuss the effective parameters of the oriented UiO-*R*-BINOL MOF. The effective parameters are calculated with the T-matrix based approach presented in[18]. In Figure S7(**a**), the diagonal elements of the effective chirality tensor are depicted. First, we observe that the chirality tensor is highly anisotropic. Second, the imaginary parts of the diagonal elements have different signs. The off-diagonal elements normalized to the *xx*-component of the effective permittivity tensor are shown in Figure S7(**b**). These terms are not negligible. Due to the anisotropy of the permittivity and the chirality tensor, the electric field is rotated during the light-matter interaction. Therefore,

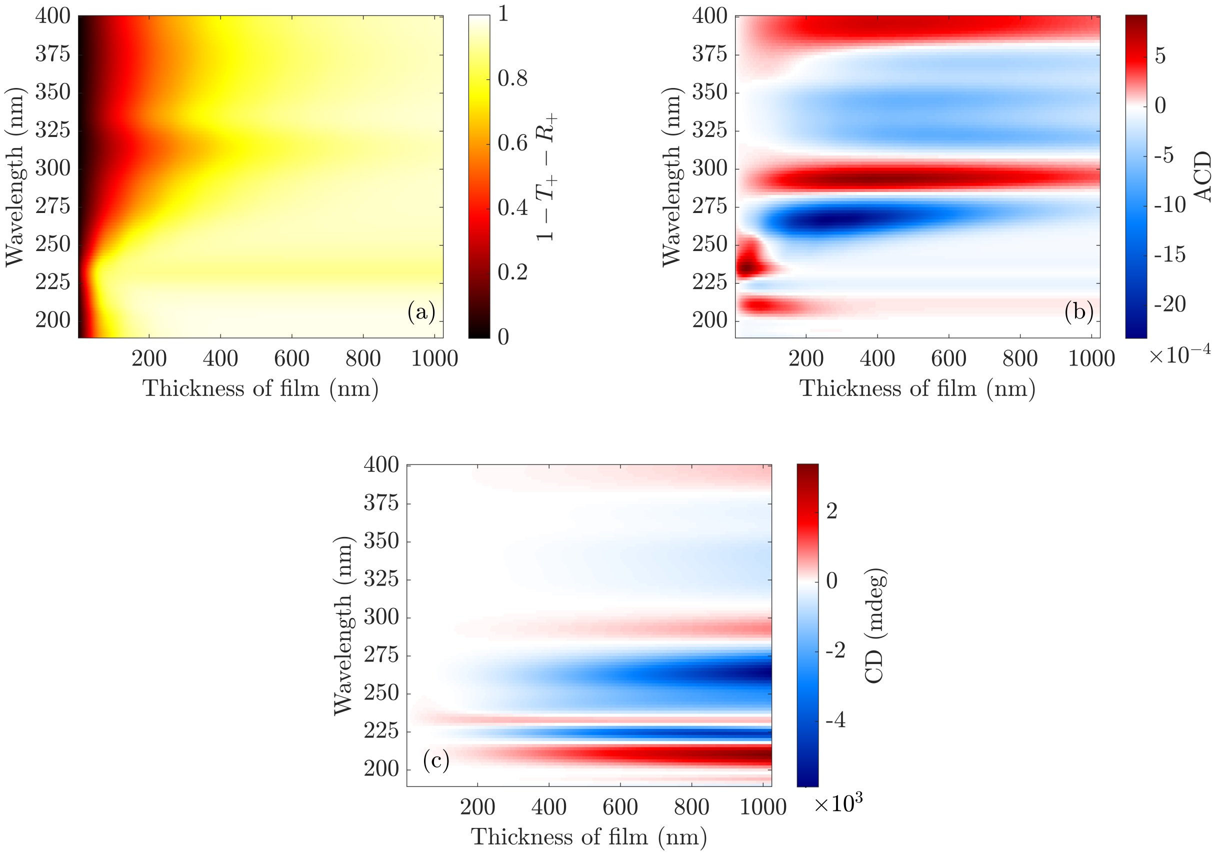


FIG. S6: Absorption **(a)**, ACD **(b)**, and CD spectra **(c)** of a UiO-*R*-BINOL film on a glass substrate. The absorption is broad and does not show distinct features. The ACD and CD spectra have the same sign in the regions of high circular dichroism. Especially, both spectra show a change of sign for wavelengths between 225 nm and 250 nm and at an approximate thickness of 200 nm.

not only the *xx* and *yy* entries but all terms of the chirality tensor influence the circular dichroism signal. The direction of the wavevector of the light does not change during the process but the polarization direction does such that not only the circular dichroism of the (effective) unit cell or the chirality tensor for a polarization in the *xy*-plane but also the other cases become important. As the imaginary part of the elements of the chirality tensor shows different signs, depending on the polarization, the circular dichroism can change its sign after a certain propagation distance. This effect can become more pronounced by larger propagation distances. We observe, therefore, in Figure S6 a sign change of the circular dichroism for some wavelengths with increasing thickness of the film. Especially for wavelengths between 225 nm and 250 nm, for which the elements of the chirality tensor strongly differ from each other and the off-diagonal terms of the permittivity

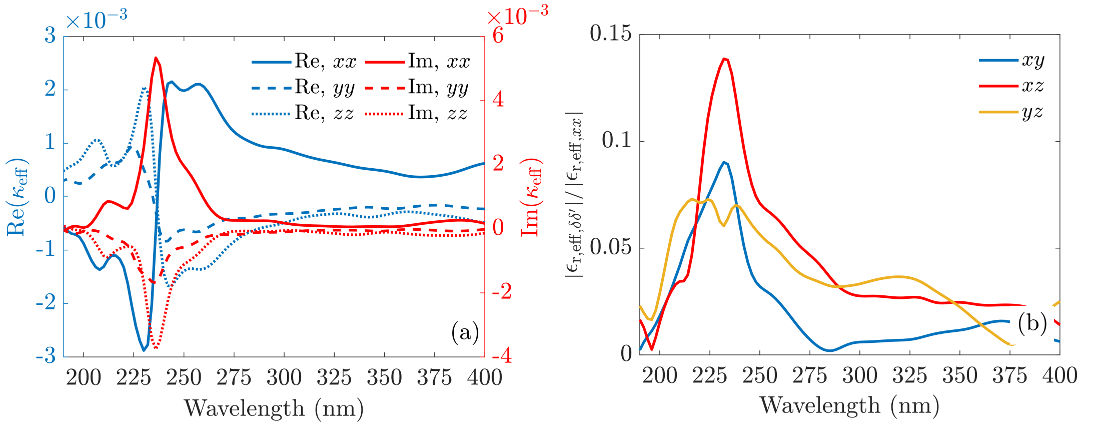


FIG. S7: Diagonal entries of effective chirality tensor **(a)**. Off-diagonal entries of effective permittivity tensor **(b)** normalized to the *xx*-component. The chirality parameter changes its sign depending on the specific polarization of the illuminating wave. The off-diagonal terms are not negligible in comparison to the diagonal terms of the effective permittivity. Due to the anisotropy of the permittivity and chirality tensor, the polarization of the field of the propagating light rotates and the field probes different terms of the chirality tensor. This effect increases for higher values of the thickness such that we observe in Figure S6 a change of the sign of the circular dichroism for wavelengths in the range between 225 nm and 250 nm, for instance.

tensor are not negligible in comparison to the diagonal terms, the circular dichroism strongly differs comparing small values of the thickness to larger values of the thickness. For larger values of the thickness, the propagation distance and therefore the rotation of the polarization direction is larger. This effect observed in the simulation can only be observed also in an experiment, in which the illuminating light spot is not much larger than the different regions of different crystalline orientations. It shows, however, that our presented methodology is able to resolve the influence of all structural properties of the analyzed molecular ensemble.

## VII. CARTESIAN COORDINATES OF MOLECULAR MODELS USED IN DFT SIMULATIONS

The Cartesian coordinates for the structures of the periodic and the molecular model of the UiO-67-*R*-BINOL MOF used in the DFT simulations and produced within this can be found deposited in the NOMAD materials database under following DOIs:

10.17172/NOMAD/2022.11.30-1
10.17172/NOMAD/2022.11.30-2

## REFERENCES


[1]T. D. Kühne, M. Iannuzzi, M. Del Ben, V. V. Rybkin, P. Seewald, F. Stein, T. Laino, R. Z. Khaliullin, O. Schütt, F. Schiffmann, D. Golze, J. Wilhelm, S. Chulkov, M. H. Bani-Hashemian, V. Weber, U. Borštnik, M. Taillefumier, A. S. Jakobovits, A. Lazzaro, H. Pabst, T. Müller, R. Schade, M. Guidon, S. Andermatt, N. Holmberg, G. K. Schenter, A. Hehn, A. Bussy, F. Belleflamme, G. Tabacchi, A. Glöß, M. Lass, I. Bethune, C. J. Mundy, C. Plessl, M. Watkins, J. VandeVondele, M. Krack, and J. Hutter, "Cp2k: An electronic structure and molecular dynamics software package - quickstep: Efficient and accurate electronic structure calculations," J. Chem. Phys. **152**, 194103 (2020).

[2]J. VandeVondele and J. Hutter, "Gaussian basis sets for accurate calculations on molecular systems in gas and condensed phases," J. Chem. Phys. **127**, 114105 (2007).

[3]S. Goedecker, M. Teter, and J. Hutter, "Separable dual-space gaussian pseudopotentials," Phys. Rev. B **54**, 1703–1710 (1996).

[4]C. Hartwigsen, S. Goedecker, and J. Hutter, "Relativistic separable dual-space gaussian pseudopotentials from h to rn," Phys. Rev. B **58**, 3641–3662 (1998).

[5]M. Krack, "Pseudopotentials for h to kr optimized for gradient-corrected exchange-correlation functionals," Theoretical Chemistry Accounts **114**, 145–152 (2005).

[6]"TURBOMOLE V7.6 2021, a development of University of Karlsruhe and Forschungszentrum Karlsruhe GmbH, 1989-2007, TURBOMOLE GmbH, since 2007; available from `https://www.turbomole.org`.".

[7]J. P. Perdew, K. Burke, and M. Ernzerhof, "Generalized gradient approximation made simple," Phys. Rev. Lett. **77**, 3865–3868 (1996).

[8]J. P. Perdew, K. Burke, and M. Ernzerhof, "Generalized gradient approximation made simple [phys. rev. lett. 77, 3865 (1996)]," Phys. Rev. Lett. **78**, 1396–1396 (1997).

[9]F. Weigend and R. Ahlrichs, "Balanced basis sets of split valence, triple zeta valence and quadruple zeta valence quality for h to rn: Design and assessment of accuracy," Phys. Chem. Chem. Phys. **7**, 3297 (2005).

[10]R. Ahlrichs, "Efficient evaluation of three-center two-electron integrals over gaussian functions," Phys. Chem. Chem. Phys. **6**, 5119–5121 (2004).

[11]M. Sierka, A. Hogekamp, and R. Ahlrichs, "Fast evaluation of the coulomb potential for electron densities using multipole accelerated resolution of identity approximation," J. Chem. Phys. **118**,

9136–9148 (2003).

[12]B. A. Jones, T. Balan, J. D. Jolliffe, C. D. Campbell, and M. D. Smith, "Practical and scalable kinetic resolution of binols mediated by a chiral counterion," Angew. Chem. Int. Ed. **58**, 4596–4600 (2019).

[13]B. A. Jones, T. Balan, J. D. Jolliffe, C. D. Campbell, and M. D. Smith, "Corrigendum: Practical and scalable kinetic resolution of binols mediated by a chiral counterion," Angew. Chem. Int. Ed. **58**, 7164–7164 (2019).

[14]K. Tanaka, S. Oda, S. Nishihote, D. Hirayama, and Z. Urbanczyk-Lipkowska, "Efficient resolution of 2,2'-dihydroxy-1,1'-binaphthalene-4,4'- and 6,6'-dicarboxylic acid by complexation with cinchonidine and brucine," Tetrahedron: Asymmetry **20**, 2612–2615 (2009).

[15]Y. Ning, T. Fukuda, H. Ikeda, Y. Otani, M. Kawahata, K. Yamaguchi, and T. Ohwada, "Revisiting secondary interactions in neighboring group participation, exemplified by reactivity changes of iminylium intermediates," Org. Biomol. Chem. **15**, 1381–1392 (2017).

[16]E. Virmani, J. M. Rotter, A. Mähringer, T. von Zons, A. Godt, T. Bein, S. Wuttke, and D. D. Medina, "On-surface synthesis of highly oriented thin metal–organic framework films through vapor-assisted conversion," J. Am. Chem. Soc. **140**, 4812–4819 (2018).

[17]N. Childress, "BLUEWHITERED," MATLAB Central File Exchange, `https://www.mathworks.com/matlabcentral/fileexchange/4058-bluewhitered` (2021), (accessed: 2021-10-10).

[18]B. Zerulla, R. Venkitakrishnan, D. Beutel, M. Krstić, C. Holzer, C. Rockstuhl, and I. Fernandez-Corbaton, "A t-matrix based approach to homogenize artificial materials," Adv. Opt. Mater. , 2201564 (2022).
